# Supplementary material for: Fully Automated Shape Analysis Based on Forest Automata
Source: arXiv:1304.5806 source file (2013-04-21)
Supplement: Supplementary file 1 [file appendix.tex]

\section{Details of Folding}\label{sec:folding_details}
In this section, we give more details on Steps 2--4 of folding of FA from Section~\ref{sec:folding_overview}.

\paragraph{Identifying entry states.}
Entry states can be identified according to the so called forking rules. 
A \emph{forking rule} is a tree automaton rule of the form $(q,a,q_1 \cdots q_m)$ where for at least two indices $1\leq i,j\leq m$, both $q_i$ and $q_j$ accept trees with a root reference labelled by an element of $J$. 
That is, there are at least two disjoint straight paths from a node of the tree labelled by $q$ to a leaf referencing an element of $J\setminus\{\src\}\cup\{n+1\}$.
Notice that due to state uniformity of $\fa$, a node has such two paths if and only if it is labelled using a forking rule. 
$q$ is then an entry state iff there is an accepting run of $\ta_\src$ 
%\todo{Is it
%really $A_j$? Why $j$? It should rather be some TA that contains the forking
%rule, no?} 
which uses a~forking rule of $q$ as the forking rule closest to the root of the accepted tree (so that it indeed labels an entry and not only a node reachable form it). 

\paragraph{Splitting $\fa$ (construction of $\splitof \fa q$).}
For every entry state $q$, the result of splitting is an FA 
$\splitof \fa q = (\ta_1^q\cdots\ta_n^q\ta_{n+1}^q,\fports)$. 
It is the same as $\fa$ up to a changed $\src$-th component 
%\todo{What is $j$?} 
and a new $(n+1)$-th component.
The new component $\ta_{n+1}^q$ will accept trees rooted by the entries that can be labelled by $q$ in some accepting run.
%\todo{... that \emph{can} be labelled by $q$ in some accepting run?}. 
It is a copy of $\ta_\src$, but its only root state is a fresh state $q'$
and it has an additional rule $(q', a, {q_1\cdots q_n})$ for every forking rule $(q , a, {q_1\cdots q_n})$ of $\fa$.
The component $\ta_{\src}^q$ is the same as $\ta_\src$ but it has all entry forking
rules of \emph{all} entry states of $\ta_\src$ removed 
%\todo{
%What is an \emph{entry} forking rule? 
%Why all entry states? Isn't the construction bound to $q$?},
and instead of those, it has the leaf rule $(q, n+1,\epsilon)$, referencing the root of the new component $\ta_{n+1}^q$.  
Notice that $\ta_\src^q$ has removed forking rules of all entry states in $\ta_s$ and $\ta_{n+1}^q$ and the $(n+1)$-th component accepts only trees the roots of which may be labelled by a forking rule of $q$. The language of $\splitof \fa q$ is therefore a subset of the language of $\fa$. It accepts only those indexed graphs where the entry $\fork$ to the knot with the signature $J\setminus\{\src\}\cup\{\fork\}$ may  be labelled by $q$.
The construction preserves the language of $\fa$ in the way that $\langof\fa = \bigcup_{q\in E}\langof{\splitof \fa q}$ where $E$ is the set of all entry states of $\ta_\src$.

\paragraph{Constructing boxes (creating $B_q$).}
Let $j_1 = n+1$ and let $j_2,\ldots,j_k$ be the elements of $J\setminus\{\src\}$ ordered by $\leq$.
For an entry state $q$,
box $B_q$ is constructed from $\splitof \fa q$ by extracting the parts of the tree components $\ta_{j_1},\ldots,\ta_{j_k}$ 
(that accept trees rooted by elements of signatures of the optimal knots), 
and by renaming their root references from $j_i$ to $i$ for each $1\leq k \leq i$. 
We assume w.l.o.g.~that for each $1\leq i \leq k$, the root state
of $\ta_{j_i}$ does not appear on the right-hand sides of any rule of $j_i$ 
(every TA can be easily transformed to satisfy this property).

We define $B_q$ as $B_q = (\hat\ta_{j_1}\ldots\hat\ta_{j_k},\hat{\fports})$ where for each
$1\leq i \leq k$,
$\hat\ta_j$ is a copy of $\ta_{j_i}^q$ up to that we modify its root rules
(rules that lead from a root state). 
%The goal is that $\hat\ta_{j_i}$ accepts only those parts of trees of $\langof{\ta_{j_j}^q}$ that correspond to tree segments between nodes in $J\setminus\{j\}\cup\{n+1\}$ (according to Lemma~\ref{}).
We thus split the set of rule-terms $S$ of every root rule $\rule = r \rightarrow S$ of $\ta_{j_i}^q$ into the \emph{core} $S_C\subseteq S$ and the \emph{residuum} $S_R = S\setminus S_C$. The core is the set of rule-terms $a(q_1\cdots q_m)\in S$ such that for at least one index $1\leq i\leq m$, $\qspanof{q_i}$ contains an element of $J\setminus\{\src\}\cup\{n+1\}$. 
That means that the rule segment is important for connecting a tree-segment of knots that we are closing into $B_q$ to the sources of the knots.
%The core contains the sub-terms of nodes labeled by $r$ included in the tree segments. 
We thus keep only the core and remove the residuum, that is, we replace $\delta$ by the rule $r\rightarrow S_C$. 

The sequence $\hat\fports$ of port indices is a subsequence $m_1\cdots m_l$ of $1\cdots k$ which contains the index $i$ iff $j_i$ is an element of the border of a knot enclosed in the box, that is, iff there is $x\not\in\nset n\setminus \{j_1,\ldots,j_k\}$ such that either $\ta_{j_i}^q$ is referenced from $\ta_x^q$ or $\ta_x^q$ references $\ta_{j_i}$.

\paragraph{Applying boxes (construction of $\fa_q$).}
%In this step, the box $B$ to hide a part of $\splitof \fa q$ in order to decrease indegrees of joins of graphs from its language.
We create the FA $\fa_q$ which is the same as $\splitof \fa q$ up to that for every
$j\in \{j_1,\ldots,j_k\}$, all root rules $r\rightarrow S$ of $\ta_\src^q$ are replaced by
$r\rightarrow S_R\cup\{B_q(r_1,\ldots,r_m)\}$. 
In the sequence $r_1,\ldots,r_m$, every  $r_i,1\leq i \leq m$, is a
%\todo{$\leq l$?} is a
fresh state with the only (leaf) rule $(r_i,j_{m_i},\epsilon)$ that labels a
leaf by the root reference to the root of the $j_{m_i}$-th tree of $\fa_q$, so
that the graphs in $\langof B$ are connected to the nodes of graphs in
$\langof{\fa_q}$ 
%\todo{What is $\fa_g$?} 
in the right way. 

%\paragraph{The result of the operation folding}
%By this construction, we get the FA $\fa''$ such that $\semof{\fa''} = \semof\fa$.
%The sum of indegrees of joins within a graph of $\langof{\fa''}$ is smaller than the sum of indegrees of a graph of $\langof\fa$. 
%The tree automata of $\fa''$ of which accepted trees have roots that are no more joins in the encoded graphs (this can happen to $j$th component for any $j\in J$) are the eliminated by transforming $\fa''$ into the state uniform (canonicity respecting) form.

%%%%%%%%%%%%%%%%%%%%%%%%%%%%%%%%%%%%%%%%%%%%%%%%%%%%%%%%%%%%%%%%%%%%%%%%%%%%%%%%
\section{Symbolic Execution}\label{sec:symb_exec}
%%%%%%%%%%%%%%%%%%%%%%%%%%%%%%%%%%%%%%%%%%%%%%%%%%%%%%%%%%%%%%%%%%%%%%%%%%%%%%%%

For each operation $\code{op}$ in the intermediate representation of the analysed program,
the semantics of C implies the function $f_{\code{op}}$ which, when applied to the io-graph $(g,
\stackframe)$, gives the io-graph $f_{\code{op}}((g, \stackframe))$
representing the heap after executing $\code{op}$ in the following way (we fix
the stack frame edge $\stackframe \to S$).
Pointer updates of the form $\code{x = y}$, $\code{x = y\text{\texttt{->}}sl}$,
or $\code{x = null}$ replace the edge $\stackframe \to S$ with the edge
$\stackframe \to (S \setminus \{x(v_x)\}) \cup \{x(v_x')\}$, where $y(v_x') \in
S$ (for $\code{x = y}$), $y(v_y) \in S \wedge v_y \to R_y \wedge \code{sl}(v_x')
\in R_y$ (for $\code{x = y\text{\texttt{->}}sl}$), or $v_x' = \nil$ (for
$\code{x = null}$).
Updates of the form $\code{x\text{\texttt{->}}sl} = y$ replace the edge $v_x \to
R_x$, where $x(v_x) \in S$ with the edge $v_x \to (R_x \setminus
\{\code{sl}(v_{\code{sl}})\}) \cup \{\code{sl}(v_\code{sl}')\}$, where
$y(v_{\code{sl}}') \in S$.
Further, $\code{malloc(x)}$ replaces the edge $\stackframe \to S$ with the edge
$\stackframe \to (S \setminus \{x(v_s)\}) \cup \{x(v_{\mathit{new}})\}$, where
$v_{\mathit{new}}$ is a newly created node, $v_{\mathit{new}} \not\in \domof{g},
\ell(v_{\mathit{new}}) = \emptyset$.
$\code{free(x)}$ removes the node $v_x$ such that $x(v_x) \in S$ and replaces
all edges $v \to R$ with edges $v \to R \setminus \{r(v_x)\}$, thus making all
selectors pointing to $v_x$ undefined.
Data updates $\code{x\text{\texttt{->}}data = d_{\mathit{new}}}$ replace the
edge $\stackframe \to S$, where $(\code{data}, \code{d_{\mathit{old}}})(\epsilon) \in
S$, with the edge $\stackframe \to (S \setminus \{(\code{data},
\code{d_{\mathit{old}}})(\epsilon)\}) \cup \{(\code{data},
\code{d_{\mathit{new}}})(\epsilon)\}$.
Evaluating a guard $g$ on an~io-graph $(g, \stackframe)$ amounts to a test of equality
of nodes or equality of data fields of nodes.
